# Supplementary material for: Learning from Students: Applying t-Distributions to Explore Accurate and Efficient Formats for LLMs
Source: arXiv:2405.03103 source file (2024-06-10)
Supplement: Supplementary file 1 [file tab-llama2b.tex]

\begin{table}[t]
\centering
\footnotesize
\small
\setlength{\tabcolsep}{2pt}
\begin{tabular}{@{}rrrrrrr@{}} % Adjusted for the correct number of columns
\toprule
Metric & \textbf{LAMB} & \textbf{Hella} & \textbf{Wino} & \textbf{PIQA} & \textbf{BoolQ} & \textbf{ARC-c} \\
\midrule
FP32 & 73.92 & 57.14 & 69.14 & 78.07 & 77.74 & 43.43 \\
\midrule
NF4 & 72.50 & 55.22 & 66.54 & 76.66 & 74.28 & 40.70 \\
SF4 & 71.90 & 55.09 & 66.06 & 77.04 & 75.35 & 41.04 \\
\midrule
INT4 & 70.35 & 54.07 & 65.43 & 75.79 & 68.90 & 39.85 \\
\midrule
I-E2M1 & 70.39 & 53.92 & 66.22 & 76.28 & 72.11 & 39.33 \\
B-E2M1 & 70.44 & 53.73 & 64.96 & 75.03 & 69.88 & 39.51 \\
E2M1 & 72.21 & 55.10 & 65.90 & 76.93 & 74.71 & 41.38 \\
\texttt{+} SR & 64.25 & 47.97 & 61.33 & 73.01 & 68.96 & 34.47 \\
\texttt{+} SP & 72.44 & 55.30 & 66.22 & 76.39 & 74.25 & 41.98 \\
E3M0 & 66.74 & 51.16 & 64.25 & 75.68 & 71.71 & 36.18 \\
\midrule
APoT4 & 71.82 & 54.87 & 66.22 & 76.39 & 73.76 & 40.36 \\
\texttt{+} SP & 71.78 & 55.13 & 65.75 & 77.37 & 73.94 & 39.93 \\
\bottomrule
\end{tabular}%
\vspace{-5pt}
\caption{\textbf{Performance Evaluation across Various Benchmarks (Llama2-7B	W4A4 SQ (SC=128))} -- The table showcases the performance of different metrics across benchmarks.}
\label{tab:llama_gptq}
\end{table}
