# Supplementary material for: Learning from Students: Applying t-Distributions to Explore Accurate and Efficient Formats for LLMs
Source: arXiv:2405.03103 source file (2024-06-10)
Supplement: Supplementary file 2 [file tab-clipping-sweep.tex]

\begin{table}[t]
\centering
\footnotesize
\setlength{\tabcolsep}{2.7pt}
\begin{tabular}{@{}cllllllll@{}}
\toprule
\textbf{Clip} & \textbf{0.85} & \textbf{0.90} & \textbf{0.95} & \textbf{1.0} & \textbf{1.05} & \textbf{1.10} & \textbf{1.15} & \textbf{Max} \\
\midrule
NF4       & \textbf{60.60} & 60.02 & 56.04 & 57.24 & 55.26 & 52.92 & 52.84 & \textbf{60.60} \\
SF4       & 61.46 & 62.71 & 62.31 & \textbf{62.90} & 60.98 & 59.07 & 57.46 & \textbf{62.90} \\
\midrule
INT4      & 35.27 & 37.99 & 37.94 & 35.98 & 41.96 & \textbf{44.64} & 42.85 & \textbf{44.64} \\
\midrule
E2M1      & 59.02 & 58.55 & 58.58 & 54.24 & 57.44 & \textbf{59.07} & 57.51 & \textbf{59.07} \\
+ SR      & 57.47 & 60.45 & 59.07 & 59.07 & 59.07 & 59.07 & \textbf{61.46} & \textbf{61.46} \\
+ SP      & \textbf{60.32} & 58.07 & 58.28 & 54.38 & 57.74 & 58.45 & 57.00 & \textbf{60.32} \\
E3M0      & 48.96 & 47.48 & 46.26 & 49.74 & 49.61 & \textbf{50.30} & 50.11 & \textbf{50.30} \\
\bottomrule
\end{tabular}%
\caption{\textbf{ResNet18 Clipping Sweep --} The fairest datatype comparison involves a clipping sweep since each datatype has different optimal clipping thresholds.}
\label{tab:clipping}
\end{table}
