# Supplementary material for: Learning from Students: Applying t-Distributions to Explore Accurate and Efficient Formats for LLMs
Source: arXiv:2405.03103 source file (2024-06-10)
Supplement: Supplementary file 3 [file tab-smoothquant.tex]

\begin{table}[t]
\centering
\footnotesize
\setlength{\tabcolsep}{4pt} % Adjusted for better spacing
\begin{tabular}{@{}rrrrr@{}} 
\toprule
 & \multicolumn{2}{c}{\textbf{Channelwise}} & \multicolumn{2}{c}{\textbf{Subchannel}} \\
 & \textbf{No SQ} & \textbf{SQ} & \textbf{No SQ} & \textbf{SQ} \\
\midrule
NF4         & -41.87 & -22.30 & \textbf{-2.65} & -3.60 \\
SF4         & \textbf{-25.12} & \textbf{-14.02} & -2.82 & \textbf{-3.45} \\
\cmidrule{1-5}
INT4        & -52.01 & -50.42 & -6.27 & -6.35 \\
\cmidrule{1-5}
E2M1-I      & -51.63 & -51.69 & -6.11 & -5.60 \\
E2M1-B      & -52.68 & -52.71 & -7.47 & -6.63 \\
E2M1        & -37.01 & -20.93 & \textbf{-2.68} & -3.44 \\
+ SR        & -25.04 & -20.88 & -12.28 & -13.14 \\
+ SP        & -41.16 & \textbf{-20.03} & -3.42 & \textbf{-3.24} \\
E3M0        & \textbf{-16.17} &  \textbf{-23.46}   & -10.66 & -9.13       \\
\cmidrule{1-5}
APoT4        & \textbf{-51.19} & -48.89  & -3.74 &  -4.23      \\
+ SP        & -51.39 & -42.49      & \textbf{-3.50} &   \textbf{-4.19 }    \\
\bottomrule
\end{tabular}
\caption{\textbf{LlaMA2-7B W4A4 SmoothQuant} -- Quality differences between formats are not changed with adding SmoothQuant~(SQ). Results use either channelwise or subchannel quantization with a subchannel block size of 128. The average accuracy drop (\%) is shown, calculated across LAMBADA, HellaSwag, Winogrande, PIQA, BoolQ, and ARC-c. Activation quantization is dynamic and SQ uses an alpha factor of 0.5.}
\label{tab:smoothquant}
\end{table}
